# Supplementary material for: Federated Contrastive Learning of Graph-Level Representations
Source: arXiv:2411.12098 source file (2024-11-18)
Supplement: Supplementary file 1 [file appendix.tex]

\newpage
\onecolumn
\appendix

\section{Details for Experimental Setup}

% \subsection{FCLG Hyper-parameter Settings}
\label{FCLG hyper-parameter}

Detailed experimental settings are provided in Table~\ref{tab: FCLG datasets hyper-parameters}. Here $\tau$ and $\tau^{\prime}$ are the temperature parameters for the intra-contrasting and inter-contrasting respectively. $\alpha$ is the teleport probability in the diffusion mechanism when constructing the augmentation view.

\begin{table}
    \centering
    \caption{ FCLG hyper-parameter settings on 4 datasets}
    \begin{adjustbox}{width=0.6\textwidth}
    \begin{tabular}{lrrrr}
    \hline
    Hyper-parameters & PROTEINS & ENZYMES & DHFR & NCI1  \\
    \hline
    learning\_rate  & $ 1e-3 $  & $ 1e-5 $  & $ 1e-4 $  & $ 1e-4 $   \\
    num\_layers    & 2  & 4   & 5   & 5   \\
    num\_neuron    & 128   &  256   & 256   & 32   \\
    batch\_size & 128 &  128 &  128  & 64   \\
    $\tau$  & $ 1e2 $   & $ 1.0 $   & $ 1.0 $   & $ 1e-2 $    \\
    $\tau^{\prime}$ & $ 0.5 $ & $ 1.0 $ & $ 1.0 $ & $ 0.5 $   \\
    $\alpha$ & $ 0.05 $   & $ 0.1 $   & $ 0.2 $   & $ 0.2 $   \\
    local\_epochs  & $ 20 $   & $ 10 $  & $ 40 $   & $ 5 $   \\
    communicate\_rounds & $ 20 $  & $ 20 $  & $ 20 $   & $ 20 $   \\
    \hline
    \end{tabular}
    \end{adjustbox}
    \label{tab: FCLG datasets hyper-parameters}
\end{table}

\section{Baseline resources}

All baseline codes used are summarized  in Table~\ref{tab:baseline codes}.

\begin{table}[tbh]
\begin{small} 
    \centering
    \caption{URLs of reference and baseline codes}
    \label{tab:baseline codes}
   \begin{adjustbox}{width=0.75\columnwidth,center}
    \begin{tabular}{cl}
    \hline
    Framework  & URL \\
    \hline
    InfoGraph    & \url{https://github.com/fanyun-sun/InfoGraph} \\
    MVGRL    & \url{https://github.com/kavehhassani/mvgrl} \\
    GIN   & \url{https://github.com/weihua916/powerful-gnns} \\
    FedAvG    & \url{https://github.com/vaseline555/Federated-Averaging-PyTorch} \\ 
    FedProx    & \url{https://github.com/litian96/FedProx} \\
    SimCLR  & \url{https://github.com/google-research/simclr} \\
    MOON    & \url{https://github.com/QinbinLi/MOON} \\
    \hline
    \end{tabular}
   \end{adjustbox}
    \end{small} 
\end{table}
